# Supplementary material for: Heterodyne-Detected Ultrafast X-Ray Diffraction and Scattering from Nonstationary States
Source: arXiv:1611.07085 ancillary file (2016-11-21)
Supplement: Supplementary file 1 [file PRLdiffractionSI.pdf]

# Heterodyne Detected X-Ray Diffraction and Scattering from Nonstationary States
# - Supplementary Material -

Kochise Bennett, Markus Kowalewski, and Shaul Mukamel

## I. QUASI-ELASTIC X-RAY SCATTERING

In Ref. [1], we derived the following expressions for the two-molecule and single-molecule frequency-resolved diffraction signals

$$S_2(\bar{\omega}, \mathbf{k}_s, \Lambda) = \int d\omega |\mathcal{F}_f(\omega, \bar{\omega})|^2 \omega'^2 \sum_{\beta \neq \alpha} \sum_{\alpha} \int d\omega_p d\omega_{p'} A_p(\omega_p) A_p^*(\omega_{p'}) e^{-i(\mathbf{q}\cdot\mathbf{r}_\alpha - \mathbf{q}'\cdot\mathbf{r}_\beta)} \times \langle \hat{\sigma}_\beta(-\mathbf{q}', \omega_{p'} - \omega) \rangle \langle \hat{\sigma}_\alpha(\mathbf{q}, \omega - \omega_p) \rangle \tag{S1}$$

$$S_1(\bar{\omega}, \mathbf{k}_s, \Lambda) = \int d\omega |\mathcal{F}_f(\omega, \bar{\omega})|^2 \omega'^2 \sum_{\alpha} \int d\omega_p d\omega_{p'} A_p(\omega_p) A_p^*(\omega_{p'}) e^{-i(\mathbf{q}-\mathbf{q}')\cdot\mathbf{r}_\alpha} \times \langle \hat{\sigma}_\alpha(-\mathbf{q}', \omega_{p'} - \omega') \hat{\sigma}_\alpha(\mathbf{q}, \omega' - \omega_p) \rangle. \tag{S2}$$

In Eqs. (S1)-(S2), $A_p(\omega)$ is the vector potential envelope for the X-ray probe, $\mathcal{F}_f$ is a frequency gating (detector sensitivity) function, $\Lambda$ stands for the set of parameters defining the X-ray field, and $\mathbf{q}^{(\prime)} \equiv \frac{\omega}{c}\hat{\mathbf{k}_s} - \mathbf{k}_{p^{(\prime)}}$ is the momentum transfer ($\hat{\mathbf{k}_s}$ is the direction of the scattered wavevector). In standard applications, the molecules that compose the sample are assumed to have identical charge distributions and the subscripts $\alpha, \beta$ on the charge density should be dropped, as we will do for the remainder of this manuscript. Note however that the two-molecule nature of Eq. (S1) is no longer explicit. The recent error in Ref. [2] originated from interpreting this as a single molecule $\alpha = \beta$ contribution. This is explained further in the main text. Assuming no frequency resolution, we have $\mathcal{F}_f(\omega, \bar{\omega}) = 1$ for the frequency gating function. The long-range (inter-molecular) structure of the sample is captured by the structure factors

$$F_1(\mathbf{q}) = \sum_{\alpha} e^{-i\mathbf{q}\cdot\mathbf{r}_\alpha} \tag{S3}$$

$$F_2(\mathbf{q}, \mathbf{q}') = \sum_{\alpha} \sum_{\beta \neq \alpha} e^{-i(\mathbf{q}\cdot\mathbf{r}_\alpha - \mathbf{q}'\cdot\mathbf{r}_\beta)}$$

in terms of which the diffraction signals can be written as

$$S_1(\mathbf{k}_s,\Lambda) = \int d\omega \frac{\omega^2}{\omega_p\omega_p'} \int d\omega_p d\omega_{p'} E_p(\omega_p) E_p^*(\omega_{p'}) \times F_1(\mathbf{q}-\mathbf{q}')\langle\hat{\sigma}(-\mathbf{q}',\omega_{p'}-\omega)\hat{\sigma}(\mathbf{q},\omega-\omega_p)\rangle \tag{S4}$$

$$S_2(\mathbf{k}_s,\Lambda) = \int d\omega \frac{\omega^2}{\omega_p\omega_p'} \int d\omega_p d\omega_{p'} E_p(\omega_p) E_p^*(\omega_{p'}) \times F_2(\mathbf{q},\mathbf{q}')\langle\hat{\sigma}(-\mathbf{q}',\omega_{p'}-\omega)\rangle\langle\hat{\sigma}(\mathbf{q},\omega-\omega_p)\rangle \tag{S5}$$

where we have substituted the electric field envelopes for the vector potential. For near-elastic scattering, we approximate $\frac{\omega}{\omega_p^{(\prime)}} \approx 1$, which is nearly valid even for inelasticities of several eV since the central frequency of the X-ray pulse is on the order of 10keV. Similarly, the momentum transfer is approximated as independent of frequency. For the purposes of time-resolved diffraction studies, a time-domain expression is more convenient to simulate due to the nuclear motion. We thus substitute the time-domain charge density operator

$$\hat{\sigma}(\mathbf{q},\omega) = \int dt \hat{\sigma}(\mathbf{q},t)e^{i\omega t}, \tag{S6}$$

where we work in the interaction picture so that the operator time-dependence is through the field-free propagator, to obtain

$$S_2(\mathbf{q},\Lambda) = F_2(\mathbf{q},\mathbf{q}) \int d\omega \int dt dt' e^{i\omega(t-t')} E_p(t) E_p^*(t')\langle\hat{\sigma}(-\mathbf{q},t')\rangle\langle\hat{\sigma}(\mathbf{q},t)\rangle \tag{S7}$$

$$S_1(\mathbf{q},\Lambda) = F_1(0) \int d\omega \int dt dt' e^{i\omega(t-t')} E_p(t) E_p^*(t')\langle\hat{\sigma}(-\mathbf{q},t')\hat{\sigma}(\mathbf{q},t)\rangle \tag{S8}$$

where we have replaced $\mathbf{k}_s$ by $\mathbf{q}$ in the argument in accordance with the quasi-elastic approximation.. Upon carrying out the $d\omega$ integration and using $\hat{\sigma}(-\mathbf{q}) = \hat{\sigma}^*(\mathbf{q})$, finally results in

$$S_2(\mathbf{q},\Lambda) = F(\mathbf{q}) \int dt |E_p(t)|^2 |\langle\hat{\sigma}(\mathbf{q},t)\rangle|^2 \tag{S9}$$

$$S_1(\mathbf{q},\Lambda) = N \int dt |E_p(t)|^2 \langle|\hat{\sigma}(\mathbf{q},t)|^2\rangle. \tag{S10}$$

For simplicity, we have relabeled $F_2(\mathbf{q},\mathbf{q}) \to F(\mathbf{q})$ here and in the main text since, under the above approximations, $F_2$ is diagonal in $\mathbf{q}$ and $F_1$ only contributes at $F_1(0) = N$. Using the time-dependent wavefunction given by the direct product of a normalized nuclear wavepacket $|\chi\rangle$ and electronic states $|\phi_i\rangle$ with amplitudes $c_i$

$$|\Psi(t)\rangle = \sum_{i=e,g} c_i(t)|\chi_i(t)\rangle \otimes |\phi_i\rangle \tag{S11}$$

we finally arrive at

$$S_2(\mathbf{q},t) = F(\mathbf{q})\left|\sum_{ij}\rho_{ij}(t)\langle\chi_i(t)|\hat{\sigma}_{ij}(\mathbf{q})|\chi_j(t)\rangle\right|^2 \tag{S12}$$

and

$$S_1(\mathbf{q},t) = N\sum_{ijk}\rho_{ij}(t)\langle\chi_i(t)|\hat{\sigma}^*_{ik}(\mathbf{q})\hat{\sigma}_{kj}(\mathbf{q})|\chi_j(t)\rangle \tag{S13}$$

where we have defined the electronic populations and coherences $\rho_{ij}(t) = c_i^*(t)c_j(t)$ and, for brevity, omitted the integration over the X-ray time envelope (and thus replaced $\Lambda$ by $t$ in the arguments of the $S_{1(2)}$). Equations (S12) and (S13) are compactly represented diagramatically by Fig. 1 in the main text. Explicitly expanding the summations yields Eqs. (7) and (8) in the main text, represented diagramatically by Fig. S1.

## II. THE ELECTRONIC CHARGE DENSITY OPERATOR

In this section, we discuss the operator nature of the charge density and its consequences. In this section, we will ignore nuclear dependence and will begin by considering a one-electron system. We seek an operator $\hat{\sigma}(\mathbf{r})$ such that the expectation value in a given state is the charge density

$$\begin{aligned}|\psi(\mathbf{r})|^2 \equiv \langle\psi|\hat{\sigma}(\mathbf{r})|\psi\rangle &= \int d\mathbf{r}'d\mathbf{r}''\langle\psi|\mathbf{r}''\rangle\langle\mathbf{r}''|\hat{\sigma}(\mathbf{r})|\mathbf{r}'\rangle\langle\mathbf{r}'|\psi\rangle \\ &= \int d\mathbf{r}'d\mathbf{r}''\psi^*(\mathbf{r}'')\psi(\mathbf{r}')\langle\mathbf{r}''|\hat{\sigma}(\mathbf{r})|\mathbf{r}'\rangle\end{aligned} \tag{S14}$$

This identifies the real-space matrix elements of the electronic charge density field operator

$$\sigma_{\mathbf{r}''\mathbf{r}'}(\mathbf{r}) \equiv \langle\mathbf{r}''|\hat{\sigma}(\mathbf{r})|\mathbf{r}'\rangle = \delta(\mathbf{r}-\mathbf{r}')\delta(\mathbf{r}-\mathbf{r}''). \tag{S15}$$

For a state decomposed into eigenmodes $|\psi\rangle = \sum_k c_i|i\rangle$, we have

$$\langle\psi|\hat{\sigma}(\mathbf{r})|\psi\rangle = \sum_{ij}\rho_{ij}\psi_i^*(\mathbf{r})\psi_j(\mathbf{r}) \tag{S16}$$

where $\rho_{ij} = c_i^*c_j$ are the electronic populations and coherences. Note that this matches the usual field-theoretic definition of the charge density $\hat{\sigma}(\mathbf{r}) = \hat{\psi}^\dagger(\mathbf{r})\hat{\psi}(\mathbf{r})$

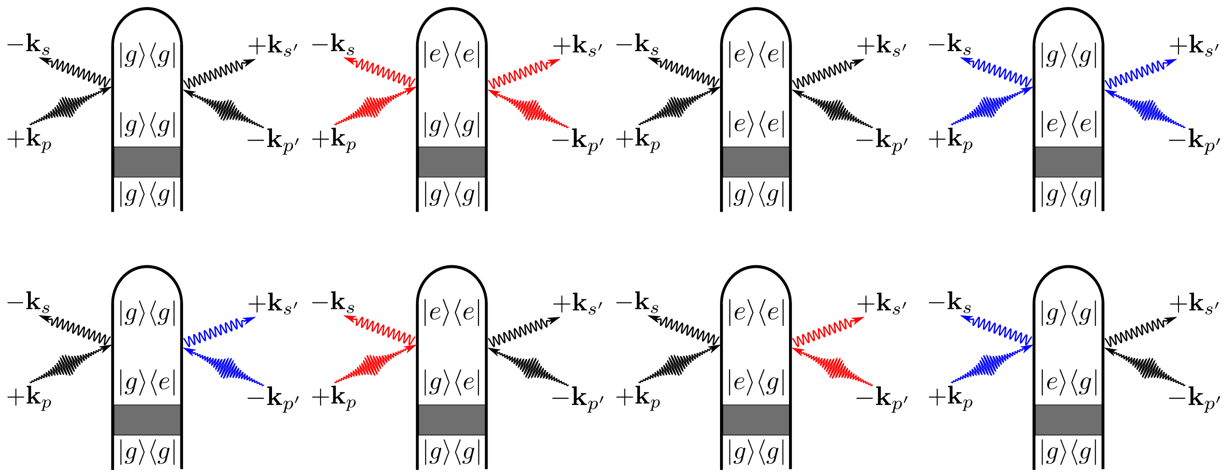


(*i*)

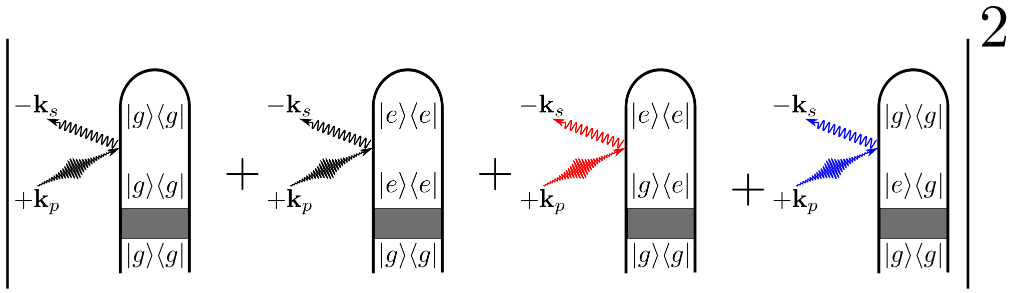


(*ii*)

FIG. S1. Loop diagrams for single-molecule (i) and two-molecule (ii) X-ray scattering processes given by Eqs. (7) and (8) in the main text. The amplitude-squared form of the two-molecule contribution is explicitly indicated. The shaded area represents an arbitrary excitation that prepares the system in a superposition state of $|g\rangle$ and $|e\rangle$. We denote modes of the X-ray probe pulse with $p$ and $p'$ whereas $s$, $s'$ represent relevant scattering modes ($\mathbf{k}_{p^{(\prime)}}$ has frequency $\omega_{p^{(\prime)}}$ and $\mathbf{k}_{s^{(\prime)}}$ has frequency $\omega_{s^{(\prime)}}$). Elastic scattering processes come with $\hat{\sigma}_{gg}$ or $\hat{\sigma}_{ee}$ and are denoted by black field arrows. Inelastic processes in which the molecule gains (Stokes) or loses (anti-Stokes) energy to the field come with $\hat{\sigma}_{ge}$ or $\hat{\sigma}_{eg}$ depending whether the action is on the ket or bra and are denoted with red and blue field arrows to indicate the field's spectral shift due to the particular diagram. Note that we use $|i\rangle$ instead of $|\phi_i\rangle$ for the electronic states in this figure to aid readability.

### A. The One-Electron Charge Density Operator of a Many-Electron System

In this section, we extend the reasoning of the previous section to an $n$-electron state $|\Psi\rangle$. The real-space identity operator in the space spanned by such states is

$$\int d\mathbf{r}_1 \dots d\mathbf{r}_n |\mathbf{r}_1, \dots, \mathbf{r}_n\rangle\langle\mathbf{r}_1, \dots, \mathbf{r}_n| \equiv \int \{d\mathbf{r}\}\big|\{\mathbf{r}\}\rangle\langle\{\mathbf{r}\}\big| \tag{S17}$$

and the one-electron charge density is [? ]

$$\int d\mathbf{r}_2 \dots d\mathbf{r}_n \big|\Psi\left(\{\mathbf{r}\}\right)\big|^2 = \langle\Psi|\hat{\sigma}(\mathbf{r})|\Psi\rangle \tag{S18}$$
$$= \int \{d\mathbf{r}'\}\{d\mathbf{r}''\}\Psi^*(\{\mathbf{r}''\})\Psi(\{\mathbf{r}'\})\langle\{\mathbf{r}''|\hat{\sigma}(\mathbf{r})|\{\mathbf{r}'\}\rangle$$

Since the charge-density operator is a one-electron operator, we have the straightforward $n$-electron generalization of Eq. (S15)

$$\langle\{\mathbf{r}''|\hat{\sigma}(\mathbf{r})|\{\mathbf{r}'\}\rangle = \sum_m \delta(\mathbf{r}-\mathbf{r}'_l)\delta(\mathbf{r}-\mathbf{r}''_l)\prod_{m\neq l}\delta(\mathbf{r}'_m-\mathbf{r}''_m) \tag{S19}$$

which is directly confirmed by substitution into Eq. (S18) and gives

$$\langle\Psi|\hat{\sigma}(\mathbf{r})|\Psi\rangle = \sum_{ij}\rho_{ij}\sigma_{ij}(\mathbf{r}) \tag{S20}$$

where we have identified

$$\sigma_{ij}(\mathbf{r}) = \int d\mathbf{r}_2 \dots d\mathbf{r}_n \Psi_i^*(\mathbf{r}_1, \dots \mathbf{r}_n)\Psi_j(\mathbf{r}_1, \dots \mathbf{r}_n) \tag{S21}$$

We note that this result can equally well be obtained by use of real-space field operators for many-electron systems as explicated by Cederbaum [3]. Moreover, Eq. (S21) is readily generalized to account for nuclear degrees of freedom $\mathbf{R}$ as

$$\hat{\sigma}_{ij}(\mathbf{r}) = \int d\mathbf{r}_2 \dots d\mathbf{r}_n \Psi_i^*(\mathbf{R}, \mathbf{r}_1, \dots \mathbf{r}_n)\Psi_j(\mathbf{R}, \mathbf{r}_1, \dots \mathbf{r}_n) \tag{S22}$$

where the circumflex indicates that the left hand side remains an operator in the nuclear subspace due to dependence on $\mathbf{R}$

## ELECTRONIC STRUCTURE CALCULATION OF NAI

The electronic structure of Sodium Iodide is calculated at the CAS(6/8)/MRCI/QZP-DKH [4, 5] level of theory in all electron calculation for an inter nuclear distance of $R = 2.5$ Å.

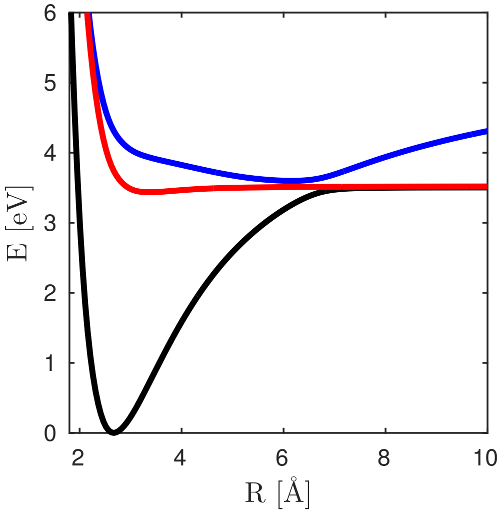


FIG. S2. Potential energy curves of NaI. $X^1\Sigma^+$ (black), $A^1\Sigma^+$ (blue), $B^1\Pi$ (red).

with program package MOLPRO [6]. The h-polarization functions on I have been removed for convenience. To account for relativistic effects caused by the Iodine core electrons a a Douglas-Kroll-Hess 10th order correction has been used [7, 8]. All densities are evaluated from the state specific density matrices in the atomic orbital basis.

The respective potential energy curves are shown in Fig. S2. The avoided curve crossing between the $X^1\Sigma^+$ state and the $A^1\Sigma^+$ state is recovered, indicating that the relativistic corrections are sufficient to recover the qualitative features of NaI.

Figure shows the three relevant components of the densities projected onto the molecular axis.


[1] K. Bennett, J. D. Biggs, Y. Zhang, K. E. Dorfman, and S. Mukamel, J. Chem. Phys. **140**, 204311 (2014).

[2] J. Glownia, A. Natan, J. Cryan, R. Hartsock, M. Kozina, M. Minitti, S. Nelson, J. Robinson, T. Sato, T. van Driel, *et al.*, Phys. Rev. Lett. **117**, 153003 (2016).

[3] A. I. Kuleff and L. S. Cederbaum, Phys. Rev. Lett. **106**, 053001 (2011).

[4] F. E. Jorge, A. C. Neto, G. G. Camiletti, and S. F. Machado, J. Chem. Phys. **130**, 064108+ (2009).

[5] G. A. Ceolin, R. C. de Berrêdo, and F. E. Jorge, Theor. Chem. Acc. **132**, 1 (2013).

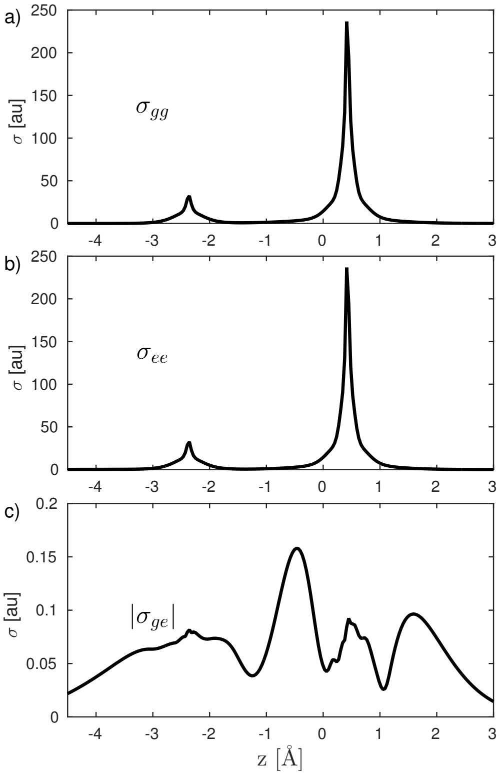


FIG. S3. Densities of NaI projected in onto the molecular axis. The densities of Na around $z = -2.35$ Å are weakly visible and dominated by the density spike of I at $z = 0.4$ Å. The projection of the transition density $\sigma_{ge}$ is obtained by integrating over its magnitude: $|\sigma_{ge}(z)| = \int\int dxdy |\sigma_{ge}(x, y, z)|$


[6] H.-J. Werner, P. J. Knowles, G. Knizia, F. R. Manby, and M. Schütz, (2015), see http://www.molpro.net.

[7] M. Douglas and N. M. Kroll, Ann. Phys.-New York **82**, 155 (1974).

[8] B. A. Hess, Phys. Rev. A **33**, 3742 (1986).
